# Supplementary material for: "Why Should You Trust My Explanation?" Understanding Uncertainty in LIME Explanations
Source: arXiv:1904.12991 source file (2019-06-04)
Supplement: Supplementary file 1 [file appendix-compas.tex]

\begin{table}
\centering
\begin{tabular}[b]{c|c|c}
    \bf black-box model &  \bf train accuracy \bf test accuracy\\
    \hline
    random forest & 0.9982 & 0.9445 \\
    gradient boosting & 0.9219 & 0.9128 \\
 
\end{tabular}
\caption{model accuracy for synthetic dataset with 8 features}
\label{tab:8feature-model-accuracy}
\end{table}

\begin{table}
\centering
\begin{tabular}[b]{c|c|c}
    \bf black-box model &  \bf train accuracy \bf test accuracy\\
    \hline
    random forest & 0.9988 & 0.9680 \\
    gradient boosting & 0.9902 & 0.972 \\
 
\end{tabular}
\caption{model accuracy for synthetic dataset with 4 features}
\label{tab:4feature-model-accuracy}
\end{table}

\begin{table}
\centering
\begin{tabular}[b]{c|c|c}
    \bf sub-dataset &  \bf train accuracy \bf test accuracy\\
    \hline
    atheism \& christian & 1.0 & 0.9066 \\
    electronic \&  crypt & 1.0 & 0.9214 \\
 
\end{tabular}
\caption{model accuracy for two-class text classification}
\label{tab:mnb-text-clf-model-accuracy}
\end{table}
