# Supplementary material for: "Why Should You Trust My Explanation?" Understanding Uncertainty in LIME Explanations
Source: arXiv:1904.12991 source file (2019-06-04)
Supplement: Supplementary file 2 [file appendix-nlp.tex]

\begin{figure*}
  \centering
  \begin{subfigure}[b]{0.49\textwidth}
    \centering
    \includegraphics[width=\linewidth]{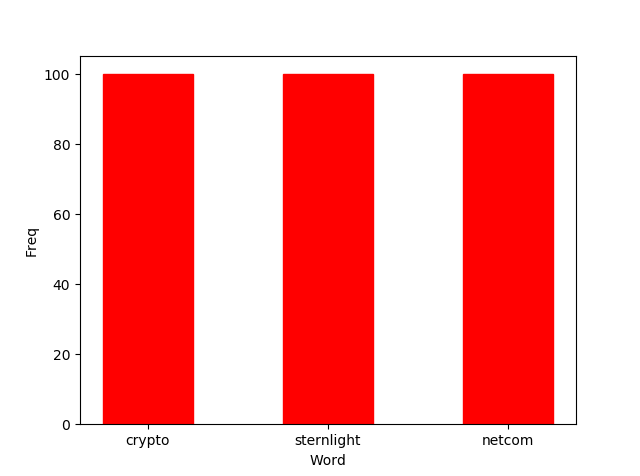}
    \caption{Test document 1}
 \label{fig:nlp-feature-counts.png}
  \end{subfigure}
  ~
  \begin{subfigure}[b]{0.49\textwidth}
    \centering
   \includegraphics[width=\linewidth]{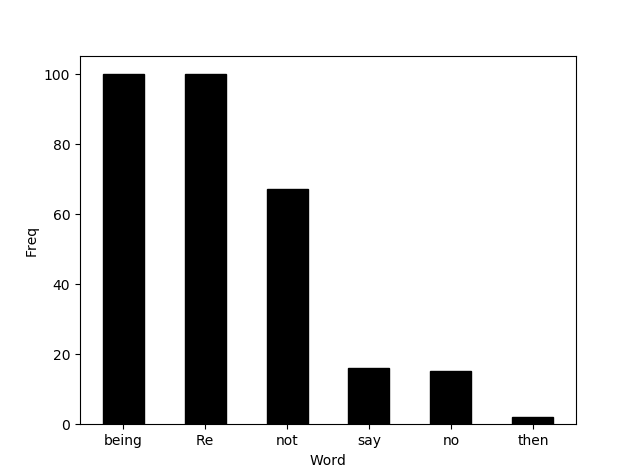}
   \caption{Test document 2}
    \label{fig:nlp-feature-counts-2.png}
  \end{subfigure}
 \caption{Frequency of important feature words in 100 iterations of explanation for text classification of "electronics" and "crypt". Words that are indicative are marked red.}
  \label{fig:mnb-nlp-2}
\end{figure*}
