# Supplementary material for: "Why Should You Trust My Explanation?" Understanding Uncertainty in LIME Explanations
Source: arXiv:1904.12991 source file (2019-06-04)
Supplement: Supplementary file 3 [file appendix-simu-more-result.tex]

\begin{figure*}
  \centering
  \begin{subfigure}[b]{0.3\textwidth}
    \centering
    \includegraphics[width=\linewidth]{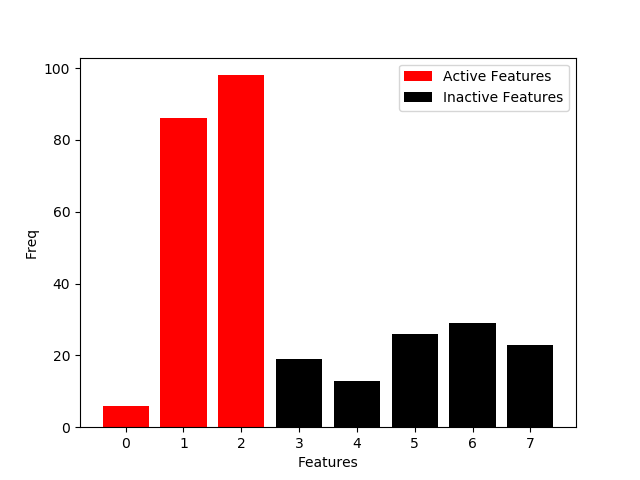}
    \caption{Leaf 0}
    \label{fig:8-label0-G}
  \end{subfigure}
  ~
  \begin{subfigure}[b]{0.3\textwidth}
    \centering
    \includegraphics[width=\linewidth]{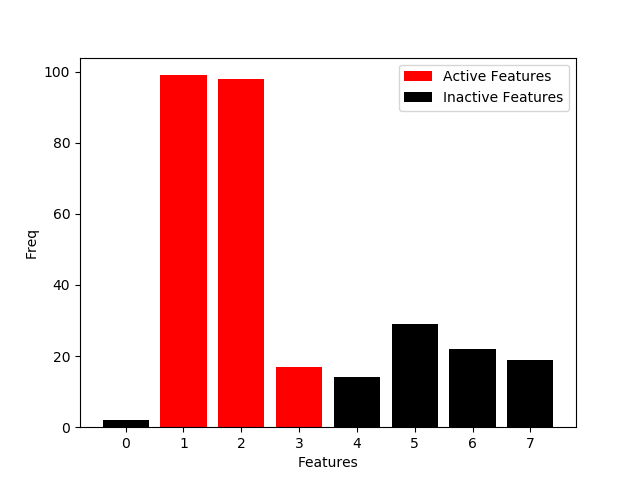}
    \caption{Leaf 1}
    \label{fig:8-label1-G}
  \end{subfigure}
  ~
  \begin{subfigure}[b]{0.3\textwidth}
    \centering
    \includegraphics[width=\linewidth]{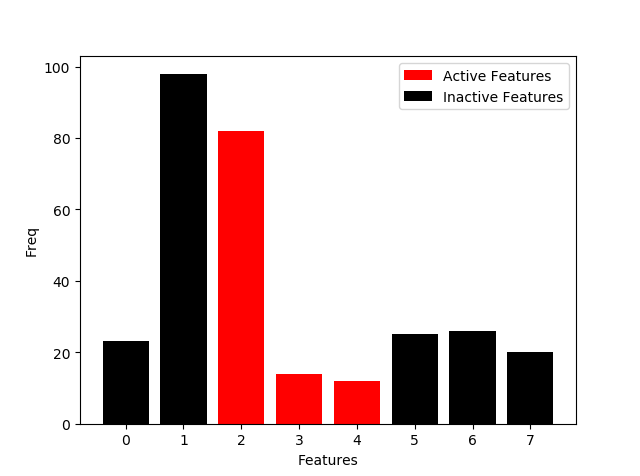}
    \caption{Leaf 2}
    \label{fig:8-label2-G}
  \end{subfigure}

  \begin{subfigure}[b]{0.3\textwidth}
    \centering
    \includegraphics[width=\linewidth]{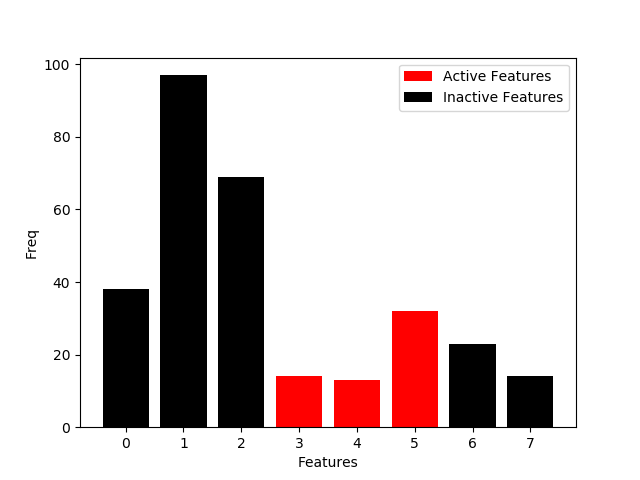}
    \caption{Leaf 3}
    \label{fig:8-label3-G}
  \end{subfigure}
  ~
  \begin{subfigure}[b]{0.3\textwidth}
    \centering
    \includegraphics[width=\linewidth]{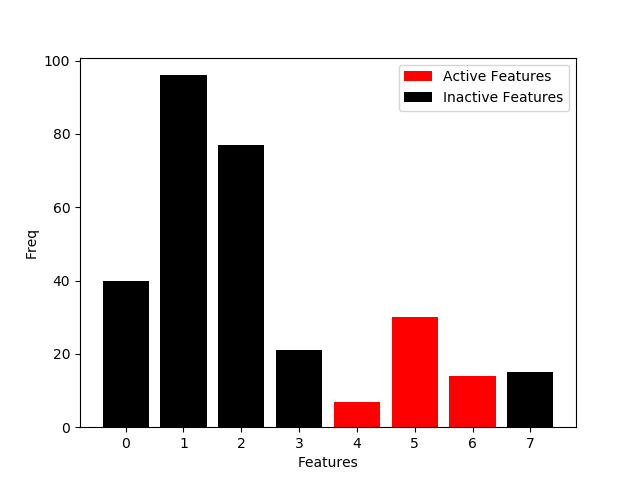}
    \caption{Leaf 4}
    \label{fig:8-label4-G}
  \end{subfigure}
  ~
  \begin{subfigure}[b]{0.3\textwidth}
    \centering
    \includegraphics[width=\linewidth]{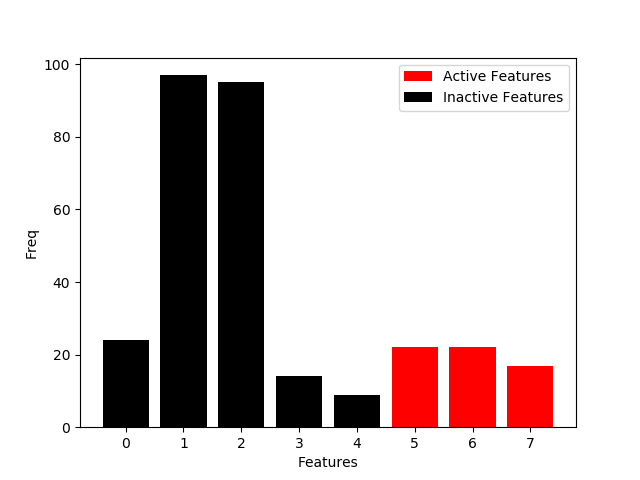}
    \caption{Leaf 5}
    \label{fig:8-label5-G}
  \end{subfigure}
  \caption{Feature frequency v.s. feature index bar plot. We picked one sample for each leaf, using lime to explain the prediction of random forest model we have trained for 100 iterations and counted the occurrence of three most important features. We marked the actual features with coefficient 1 as red bars in these plots.}
  \label{fig:8-feature-GBT}
\end{figure*}

\begin{figure*}
  \centering
  \begin{subfigure}[b]{0.3\textwidth}
    \centering
    \includegraphics[width=\linewidth]{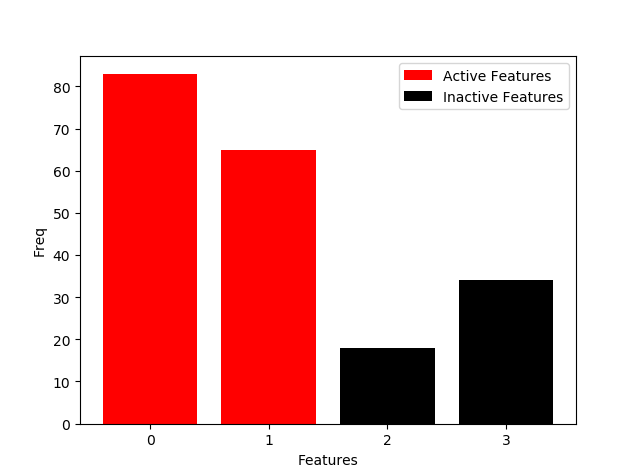}
    \caption{Leaf 0}
    \label{fig:4-label0}
  \end{subfigure}
  ~
  \begin{subfigure}[b]{0.3\textwidth}
    \centering
    \includegraphics[width=\linewidth]{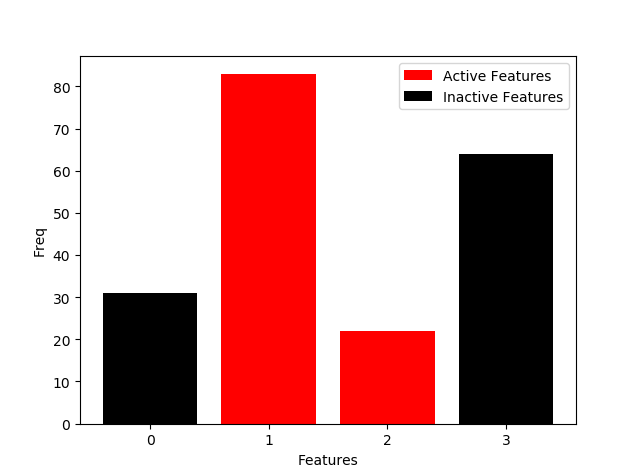}
    \caption{Leaf 1}
    \label{fig:4-label1}
  \end{subfigure}
  
  \begin{subfigure}[b]{0.3\textwidth}
    \centering
    \includegraphics[width=\linewidth]{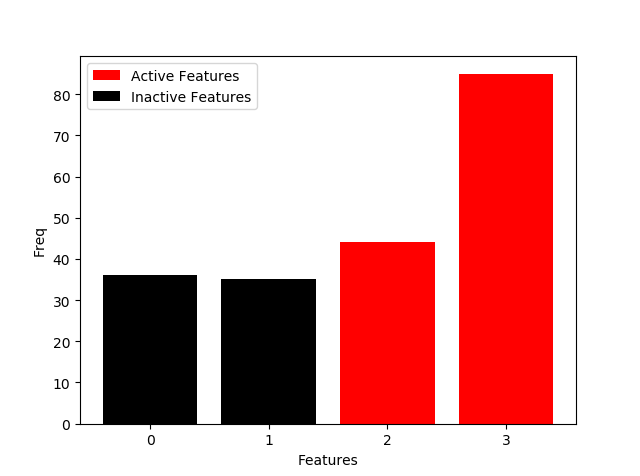}
    \caption{Leaf 2}
    \label{fig:4-label2}
  \end{subfigure}
    ~
  \begin{subfigure}[b]{0.3\textwidth}
    \centering
    \includegraphics[width=\linewidth]{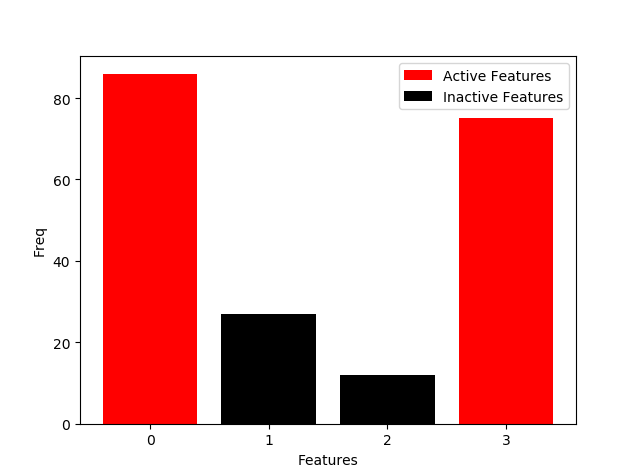}
    \caption{Leaf 3}
    \label{fig:4-label3}
  \end{subfigure}
  
  \caption{Cumulative selection frequency for four-feature synthetic data. We pick one sample in each leaf, repeat LIME 100 times to explain the prediction of the random forest model we trained, and record the two most important features in each explanation. Features with true coefficients 1 are marked red in each leaf.}
  \label{fig:random-forest-4-features}
\end{figure*}

\begin{figure*}
  \centering
  \begin{subfigure}[b]{0.3\textwidth}
    \centering
    \includegraphics[width=\linewidth]{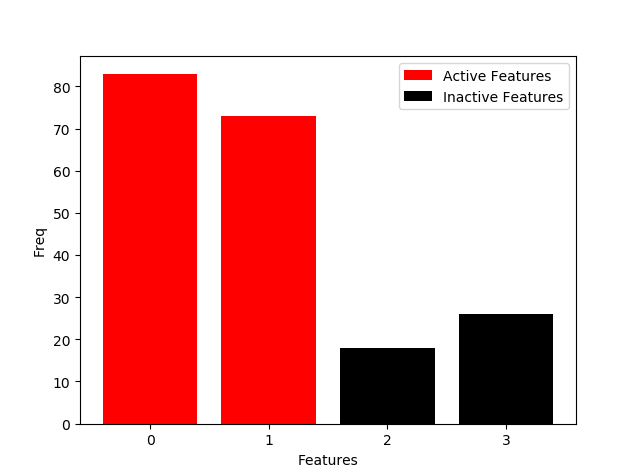}
    \caption{Leaf 0}
    \label{fig:4-label0-GBT}
  \end{subfigure}
  ~
  \begin{subfigure}[b]{0.3\textwidth}
    \centering
    \includegraphics[width=\linewidth]{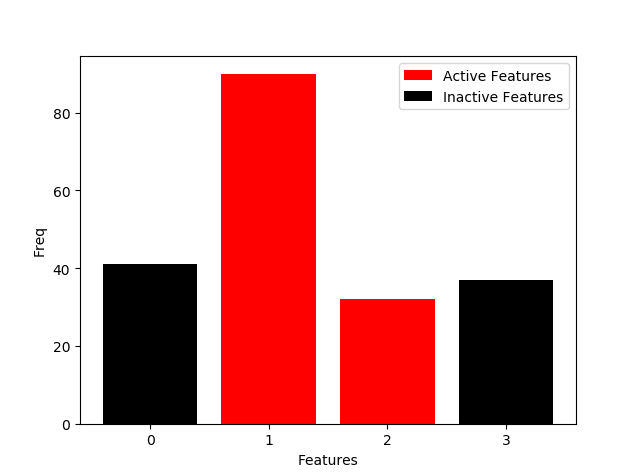}
    \caption{Leaf 1}
    \label{fig:4-label1-GBT}
  \end{subfigure}
  
  \begin{subfigure}[b]{0.3\textwidth}
    \centering
    \includegraphics[width=\linewidth]{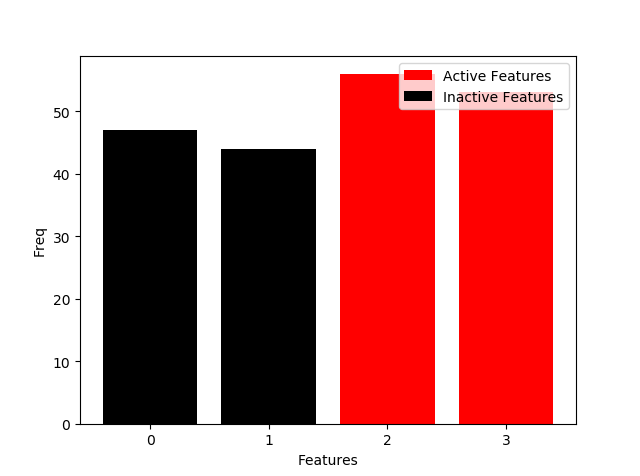}
    \caption{Leaf 2}
    \label{fig:4-label2-GBT}
  \end{subfigure}
    ~
  \begin{subfigure}[b]{0.3\textwidth}
    \centering
    \includegraphics[width=\linewidth]{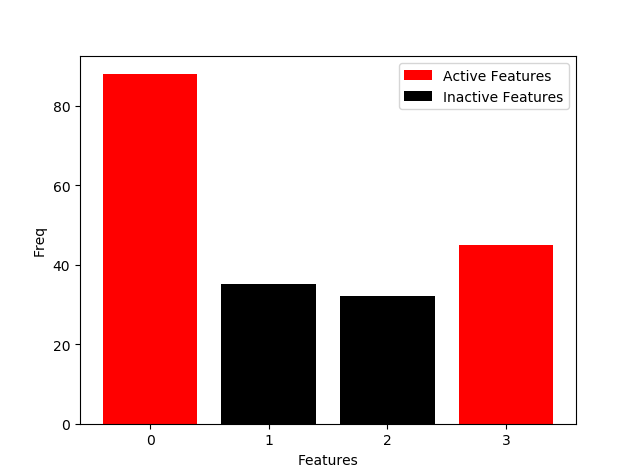}
    \caption{Leaf 3}
  \end{subfigure}
  
  \caption{The frequency v.s. most import feature index bar plots for 100 iterations of explanation for the gradient boosting classifier of 4 features synthetic data. We kept the two most important feature during each iteration.}
   \label{fig:gradient-boosting-4-features}
\end{figure*}
